# Supplementary material for: How can representation dimension dominate structurally pruned LLMs?
Source: arXiv:2503.04377 source file (2025-03-06)
Supplement: Supplementary file 1 [file limits.tex]

\subsection{Limitations and Future Work}
This paper provides precise analytical expressions between representation dimension sparsity and model performance. However, it is an optimal case that the representation dimension certainly dominates the pruned model. The reason is that the used pruning approach is SliceGPT, which reduces the representation dimension for pruning (as clarified in~\cref{fig:act_flow,tab:shape}). 
Other pruning approach, like sparsifying the sub-blocks of the weight matrices~\cite{sparsegpt} and deleting the whole layers~\cite{men2025shortgpt}, might not be as certain as the case we discussed.
